# Supplementary material for: How Uncertain Is My Action? Self-Correcting Visual Planning with Frozen World Models
Source: arXiv:2611.23620 source file (2026-11-17)
Supplement: Supplementary file 1 [file supp_labels.tex]

\makeatletter
\WarningFilter{hyperref}{Suppressing link with empty target}
\@namedef{r@alg:sp}{{S1}{}{}{}{}}
\@namedef{r@alg:sp@cref}{{[algorithm][1][]S1}{[1][1][]2}{}{}{}}
\@namedef{r@app:analysis}{{S14}{}{}{}{}}
\@namedef{r@app:analysis@cref}{{[section][14][]S14}{[1][23][]24}{}{}{}}
\@namedef{r@app:baselines}{{S12}{}{}{}{}}
\@namedef{r@app:baselines@cref}{{[section][12][]S12}{[1][20][]21}{}{}{}}
\@namedef{r@app:calibration}{{S11}{}{}{}{}}
\@namedef{r@app:calibration@cref}{{[section][11][]S11}{[1][20][]20}{}{}{}}
\@namedef{r@app:delay}{{S5.4}{}{}{}{}}
\@namedef{r@app:delay@cref}{{[subsection][4][5]S5.4}{[1][13][]13}{}{}{}}
\@namedef{r@app:dino}{{S17}{}{}{}{}}
\@namedef{r@app:dino@cref}{{[section][17][]S17}{[1][30][]30}{}{}{}}
\@namedef{r@app:estimate}{{S5.5}{}{}{}{}}
\@namedef{r@app:estimate@cref}{{[subsection][5][5]S5.5}{[1][13][]14}{}{}{}}
\@namedef{r@app:gof}{{S5.8}{}{}{}{}}
\@namedef{r@app:gof@cref}{{[subsection][8][5]S5.8}{[1][16][]16}{}{}{}}
\@namedef{r@app:identification}{{S16}{}{}{}{}}
\@namedef{r@app:identification@cref}{{[section][16][]S16}{[1][29][]29}{}{}{}}
\@namedef{r@app:lie}{{S4}{}{}{}{}}
\@namedef{r@app:lie@cref}{{[section][4][]S4}{[1][6][]6}{}{}{}}
\@namedef{r@app:limitations}{{S20}{}{}{}{}}
\@namedef{r@app:limitations@cref}{{[section][20][]S20}{[1][38][]38}{}{}{}}
\@namedef{r@app:linear}{{S6}{}{}{}{}}
\@namedef{r@app:linear@cref}{{[section][6][]S6}{[1][16][]16}{}{}{}}
\@namedef{r@app:norm}{{S5.1}{}{}{}{}}
\@namedef{r@app:norm@cref}{{[subsection][1][5]S5.1}{[1][8][]8}{}{}{}}
\@namedef{r@app:nuisance}{{S5.3}{}{}{}{}}
\@namedef{r@app:nuisance@cref}{{[subsection][3][5]S5.3}{[1][11][]11}{}{}{}}
\@namedef{r@app:protocol}{{S9}{}{}{}{}}
\@namedef{r@app:protocol@cref}{{[section][9][]S9}{[1][18][]18}{}{}{}}
\@namedef{r@app:rao}{{S5.2}{}{}{}{}}
\@namedef{r@app:rao@cref}{{[subsection][2][5]S5.2}{[1][10][]10}{}{}{}}
\@namedef{r@app:real}{{S18}{}{}{}{}}
\@namedef{r@app:real@cref}{{[section][18][]S18}{[1][30][]30}{}{}{}}
\@namedef{r@app:recovery}{{S5.6}{}{}{}{}}
\@namedef{r@app:recovery@cref}{{[subsection][6][5]S5.6}{[1][14][]14}{}{}{}}
\@namedef{r@app:recovery-details}{{S15}{}{}{}{}}
\@namedef{r@app:recovery-details@cref}{{[section][15][]S15}{[1][25][]26}{}{}{}}
\@namedef{r@app:related}{{S19}{}{}{}{}}
\@namedef{r@app:related@cref}{{[section][19][]S19}{[1][37][]37}{}{}{}}
\@namedef{r@app:shifts}{{S10}{}{}{}{}}
\@namedef{r@app:shifts@cref}{{[section][10][]S10}{[1][19][]19}{}{}{}}
\@namedef{r@app:theory-notes}{{S3}{}{}{}{}}
\@namedef{r@app:theory-notes@cref}{{[section][3][]S3}{[1][3][]3}{}{}{}}
\@namedef{r@fig:cubegrid}{{S7}{}{}{}{}}
\@namedef{r@fig:cubegrid@cref}{{[figure][7][]S7}{[1][26][]27}{}{}{}}
\@namedef{r@fig:supp-pusht-grid}{{S6}{}{}{}{}}
\@namedef{r@fig:supp-pusht-grid@cref}{{[figure][6][]S6}{[1][26][]26}{}{}{}}
\@namedef{r@lem:lan}{{S5.1}{}{}{}{}}
\@namedef{r@lem:lan@cref}{{[lemma][1][5]S5.1}{[1][10][]10}{}{}{}}
\@namedef{r@prop:confusion}{{S5.1}{}{}{}{}}
\@namedef{r@prop:confusion@cref}{{[propositionA][1][5]S5.1}{[1][16][]16}{}{}{}}
\@namedef{r@tab:attr}{{S17}{}{}{}{}}
\@namedef{r@tab:attr@cref}{{[table][17][]S17}{[1][29][]29}{}{}{}}
\@namedef{r@tab:detbase}{{S7}{}{}{}{}}
\@namedef{r@tab:detbase@cref}{{[table][7][]S7}{[1][23][]24}{}{}{}}
\@namedef{r@tab:detect}{{S5}{}{}{}{}}
\@namedef{r@tab:detect@cref}{{[table][5][]S5}{[1][22][]23}{}{}{}}
\@namedef{r@tab:ident}{{S18}{}{}{}{}}
\@namedef{r@tab:ident@cref}{{[table][18][]S18}{[1][29][]29}{}{}{}}
\@namedef{r@tab:persist}{{S13}{}{}{}{}}
\@namedef{r@tab:persist@cref}{{[table][13][]S13}{[1][27][]27}{}{}{}}
\@namedef{r@tab:supp-ablation}{{S14}{}{}{}{}}
\@namedef{r@tab:supp-ablation@cref}{{[table][14][]S14}{[1][27][]28}{}{}{}}
\@namedef{r@tab:supp-dino}{{S19}{}{}{}{}}
\@namedef{r@tab:supp-dino@cref}{{[table][19][]S19}{[1][30][]30}{}{}{}}
\@namedef{r@tab:supp-native}{{S16}{}{}{}{}}
\@namedef{r@tab:supp-native@cref}{{[table][16][]S16}{[1][28][]29}{}{}{}}
\@namedef{r@tab:supp-windows}{{S6}{}{}{}{}}
\@namedef{r@tab:supp-windows@cref}{{[table][6][]S6}{[1][22][]23}{}{}{}}
\makeatother
